# Supplementary material for: Imagine This! Scripts to Compositions to Videos
Source: arXiv:1804.03608 source file (2018-04-10)
Supplement: Supplementary file 1 [file supplementary.tex]

\noindent \textbf{Generalization to unseen videos.} An advantage of the embedding based text to entity video retrieval approach over text only methods is that the embedding approach can use any unseen video databases without any text annotations, potentially in entirely new domains (eg. learning from synthetic video caption datasets and applying the knowledge to generate real videos). Hence in Table~\ref{table:train_vs_test} we compare recall when using train set (seen) videos as the target database with recall when using test set (unseen) video as the target database. \emph{Database context} refers to whether the target embedding encodes context along with entity information or if the context has been masked out (by applying the entity segmentation mask before feeding into the target embedding network). When database context is used and previous entities are inferred (instead of GT), the recall on unseen videos is comparable to seen videos except on nouns. To investigate this further we show recalls on seen and unseen again but using GT previous entity positions and appearances. While seen database videos using GT previous entities performs comparably to inferred previous entities, recall on unseen test videos with GT previous entities is much higher than seen. This indicates that the, since the embeddings are trained using GT previous entities as queries and the corresponding whole video as target (from which the embedding of next entity is obtained using RoI pooling), both query and target embeddings share the same context. This signal is easily exploited by the triplet loss without learning semantically meaningful embeddings. To test this hypothesis we train the model without database context and find a $2.2$ point improvement in noun recall (Pred + Unseen). We also find that the gap between using GT and predicted previous entities when querying against unseen videos also shrinks from $(31.7,52.7,47.7)$ to $(24.2,43.3,43.9)$ for top-1 noun, adjective and verb recalls respectively. \\

\setlength{\tabcolsep}{3pt}
\begin{table}[t]
\begin{center}
\caption{\textbf{Generalization to Unseen Database Videos.} To help understand generalization of learned visual knowledge to unseen videos we compare entity retrieval results using test queries against seen videos (\dataset\ train) with queries against unseen videos (\dataset\ test). While context encoded using RoI pooling in both query and database embeddings performs well when querying against train set, when querying against unseen test videos we notice a significant drop when we replace GT previous entities by the predicted ones ($82.22\%$ to $50.52\%$ top-1 noun recall). We found that removing the context from the database embedding improved generalization on unseen videos ($50.52\%$ to $52.72\%$  top-1 noun recall). The gap between using GT and predicted previous entities on unseen videos is also reduced by more than 7 points.}
\label{table:train_vs_test}
\begin{tabular}{cccccccccc}
\toprule%\noalign{\smallskip}
\multirow{2}{*}{\thead{Previous \\ Entities}}  & \multirow{2}{*}{\thead{Video \\ Database}} & \multirow{2}{*}{\thead{Database \\ Context}} & \multicolumn{3}{c}{\thead{Recall@1}}   & \multicolumn{3}{c}{\textbf{Recall@10}}              \\ \cmidrule(l){4-6} \cmidrule(l){7-9}
&     &    & \thead{Noun}  & \thead{Adj.}   & \thead{Verb}      & \thead{Noun}  & \thead{Adj.}   & \thead{Verb}  \\
%\noalign{\smallskip}
\hline
\multirow{2}{*}{Pred} & Seen (Train)  & \checkmark & 61.19 & 12.36 & 14.77 & 75.98 & 47.72 & 46.86 \\
                                                      & Unseen (Test) & \checkmark & 50.52 & 11.98 & 10.4  & 69.1  & 41.25 & 42.57 \\
                                \multirow{2}{*}{GT}   & Seen (Train)  & \checkmark & 59.68 & 17.68 & 13.71 & 75.19 & 51.52 & 45.17 \\
                                                      & Unseen (Test) & \checkmark & 82.22 & 64.64 & 58.07 & 96.36 & 94.49 & 94.97 \\
                                \multirow{2}{*}{Pred} & Seen (Train)  &            & 55.89 & 13.31 & 10.03 & 72.68 & 43.73 & 42.16 \\
                                                      & Unseen (Test) &            & 52.72 & 12.17 & 8.64  & 68.61 & 37.83 & 41.38 \\
                                \multirow{2}{*}{GT}   & Seen (Train)  &            & 55.55 & 16.16 & 9.56  & 71.64 & 46.96 & 41.53 \\
                                                      & Unseen (Test) &            & 76.88 & 55.51 & 52.58 & 94.74 & 92.01 & 93.52 \\ \bottomrule
\end{tabular}
\end{center}
\end{table}
\setlength{\tabcolsep}{1.4pt}

\subsection{Turk task design (with screenshots) for metrics}
